# Supplementary material for: Atomic-scale observation of $d$-$\pi$-$d$ spin coupling in coordination structures
Source: arXiv:2501.01162 source file (2025-01-02)
Supplement: Supplementary file 1 [file SI-4.pdf]

# Supplemental Materials

## Observation of *d*-π-*d* spin coupling in metal organic coordination structure

Xue Zhang,[1,2#] Xin Li,[1#] Jie Li,[1#] Haoyang Pan,[3#] Minghui Yu,[1] Yajie Zhang,[1*] Gui-Lin Zhu,[4] Zhen Xu,[3] Ziyong Shen,[1] Shimin Hou,[1] Yaping Zang,[5] Bingwu Wang,[6] Kai Wu,[7] Shang-Da Jiang,[8] Ivano E. Castelli,[9] Lianmao Peng,[1] Per Hedegård,[10*] Song Gao,[11,8,6] Jing-Tao Lü,[4*] Yongfeng Wang[1*]

[1]Center for Carbon-Based Electronics and Key Laboratory for the Physics and Chemistry of Nanodevices, School of Electronics, Peking University, Beijing 100871, China

[2]Spin-X Institute, School of Microelectronics, State Key Laboratory of Luminescent Materials and Devices, South China University of Technology, Guangzhou 511442, China

[3]Spin-X Institute, School of Chemistry and Chemical Engineering, South China University of Technology, Guangzhou 510641, China

[4]School of Physics, Huazhong University of Science and Technology, Wuhan 430074, China

[5]BNLMS, Key Laboratory of Organic Solids, Institute of Chemistry, Chinese Academy of Sciences, Beijing 100190, China

[6]BNLMS, Beijing Key Laboratory of Magnetoelectric Materials and Devices, College of Chemistry and Molecular Engineering, Peking University, Beijing 100871, China

[7]BNLMS, College of Chemistry and Molecular Engineering, Peking University, Beijing 100871, China

[8]Spin-X Institute, School of Chemistry and Chemical Engineering, State Key Laboratory of Luminescent Materials and Devices, Guangdong-Hong Kong-Macao Joint Laboratory of Optoelectronic and Magnetic Functional Materials, South China University of Technology, Guangzhou 511442, China

[9]Department of Energy Conversion and Storage, Technical University of Denmark, DK-2800 Kongens Lyngby, Denmark

[10]Niels Bohr Institute, University of Copenhagen, DK-2100 Copenhagen, Denmark

[11]Key Laboratory of Bioinorganic and Synthetic Chemistry of Ministry of Education, School of Chemistry, IGCME, GBRCE for Functional Molecular Engineering, Sun Yat-Sen University, Guangzhou 510275, China

## 1. Theoretical details

### 1.1 DFT calculations

All calculations are carried out based on the spin-polarized framework of DFT using Vienna Ab-initio Simulation Package (VASP).[1,2] The projector augmented wave (PAW) method is employed to represent the elemental core and valence electrons, and wavefunctions are expanded using a plane-wave basis set with an energy cutoff of 450 eV.[3] The exchange-correlation potential is described using the Perdew-Burke-Ernzerh generalized gradient approximation (PBE-GGA).[4] For Fe, the GGA+U method[5] is used with $U = 5$ eV, $J = 0.9$ eV for Fe. To confirm the structure on the surface, long-range dispersion interactions are taken into consideration, which are performed using the D3-BJ method developed by Grimme.[6,7] The convergence criteria for energy and force are set to $1\times10^{-5}$ eV and 0.05 eV/Å, respectively. The stabilization of the single O atom within the chelate-site of ReA is achieved by the Au(111) surface. When dealing with gas-phase structures, during the geometry optimization process, the *y*-axis position of this single O atom is fixed, safeguarding the chelate form. Additionally, a vacuum layer of at least 15 Å along the *z*-axis is set to eliminate interactions between periodic images. For these gas-phase structures, the convergence criterion for energy has been further tightened to $1\times10^{-6}$ eV, while maintaining the force criterion at 0.05 eV/Å, ensuring both precision and stability in the calculations. The first Brillouin zone is sampled with a $\Gamma$-centered *K*-point meshs.

### 1.2 Fitting the *dI/dV* spectra based on the scattering theory

We fit the *dI/dV* spectra measured on the ReA radicals according to the scattering theory.[8] As detailed in Ref. 8, in the fitting process, the exchange energy ($C$) and the Kondo scattering term ($J_{\rho s}$) between radicals and itinerant electrons in substrate are the main parameters, and the Coulomb scattering and effective temperature are also taken into account in fitting the spectra. Besides, a linear background is used to compensate the influence of other electronic states. In the following table we show the $J_{\rho s}$ and $C$ extracted from the fitting of the spectra shown in the main text.

**Table S1.** Kondo scattering term and exchange energy between radicals and Fe atoms obtained by fitting the spectra in the main text.

| | Fig.2(b) | Fig.2(e) | Fig.3(d) W1 | Fig.3(d) W2 | Fig.3(e) | Fig.3(f) W1 | Fig.3(f) B1 | Fig.5(c) | Fig.5(d) |
|---|---|---|---|---|---|---|---|---|---|
| $J\rho_s$ | -0.668 | -1.389 | -2.285 | -1.382 | -0.400 | -0.328 | -0.162 | -0.357 | -2.342 |
| $C$(meV) | 5.09 | 1.04 | 0.36 | 0.20 | 5.50 | 0.45 | 4.81 | 5.05 | 1.16 |

## 2. Experimental details

### 2.1 Transformation of a neutral ReA molecule into a radical

We transformed a neutral ReA molecule into a radical by applying electrical pulses to the bulky 1,3,3-trimethylcyclohexene group (referred to as the head group), inducing a dehydrogenation process. Following this transformation, the head group appears brighter in the STM image. Figure S1(a) and S1(b) illustrate the changes in the STM topography before and after the transformation of a bridge-site and a wing-site ReA molecule, respectively. The tetramers shown in Fig. S1 are the same as those depicted in Fig. 2.

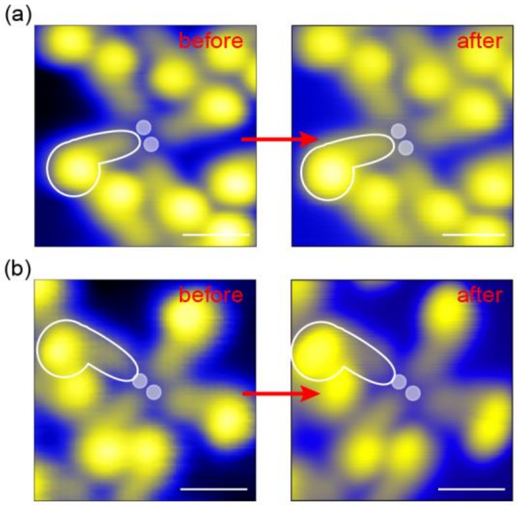


**Fig. S1 Change in the topographic height of a ReA molecule in the Fe-coordinated tetramer before and after the transformation.** (a) Transformation of a bridge-site ReA molecule. (b) Transformation of a wing-site ReA molecule. STM parameters: (a) left: $V_b$ = 30 mV, $I_{set}$ = 53 pA; right: $V_b$ = 30 mV, $I_{set}$ = 43 pA. (b) left: $V_b$ = 100 mV, $I_{set}$ = 20 pA; right: $V_b$ = 30 mV, $I_{set}$ = 53 pA.

We further transformed all four ReA molecules in a coordinated tetramer into radicals, as shown in Fig. S2(a). The *dI/dV* spectra measured on these four ReA radicals are presented in Fig. S2(b). As discussed in the main text, the magnetic coupling between the two wing-site ReA radicals via the two central Fe atoms is negligible. Consequently, the *dI/dV* spectrum of each wing-site ReA radical exhibits a single spin excitation step, which originates from the coupling with its coordinated Fe atom. In contrast, the two bridge-site ReA radicals are capable of coupling to each other through the two mutually coordinated Fe atoms. This interaction results in double spin excitation steps in the *dI/dV* spectra of both bridge-site ReA radicals, as indicated by the dashed red lines in Fig. S2(b). The inner step arises from the coupling between the bridge-site ReA radical and the two Fe atoms, while the outer step is attributed to the coupling between the two bridge-site ReA radicals.

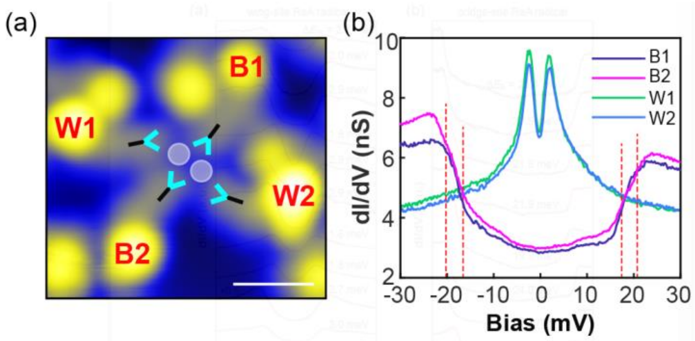


**Fig. S2 Transforming all the four ReA molecules into radicals in a Fe-coordinated tetramer.** (a) STM image of a tetramer where all the four ReA molecules were switched to be radicals. The Fe atoms (white circles) are overlapped on the images and the switched ReA molecules are marked by highlighting the schematic carboxyl groups (colored tridents). (b) d*I*/d*V* spectra measured on each transformed ReA molecule in (d). Scanning parameters: constant-current mode, $V_b$ = 30 mV, $I_{set}$ = 53 pA; *dI/dV* parameters: $V_b$ = -30 mV, $I_{set}$ = 200 pA, $V_{mod}$ = 0.6 mV.

## 2.2 Spin excitation energy of different ReA radicals coupled to Fe in the coordinated tetramer

We observe that the spin excitation energy ($\Delta E$) of a ReA radical coupled to Fe in the coordinated tetramer exhibits slight variations. For the wing-site ReA radical, $\Delta E_W$ typically falls within the range of 0.1 to 3 meV (Fig. S3(a)). In contrast, for the bridge-site ReA radical, $\Delta E_B$ generally ranges between 19 and 25 meV (Fig. S3(b)). We attribute this variation for each type of radical to subtle differences in molecular adsorption configurations, which may influence both the metal-organic interaction and the competition with molecule-substrate interaction. Despite these variations, the spin excitation energy of a wing-site ReA radical coupled to a single Fe atom consistently remains much smaller than that of a bridge-site ReA radical coupled to two Fe atoms.

## 2.3 Delocalized spin distribution of a ReA radical

The spin distribution of a ReA radical in the coordinated tetramer is delocalized along the molecular skeleton. We conducted *dI/dV* measurements at different positions on both a wing-site and a bridge-site ReA radical, as illustrated in Fig. S4(a) and S4(b). Along the molecular

skeleton, the spin excitation feature originating from *d*-π coupling exhibits an oscillatory trend for both wing-site and bridge-site ReA radicals. This observation aligns well with our DFT calculations of the spin density of a ReA radical, as shown in Fig. 1a.

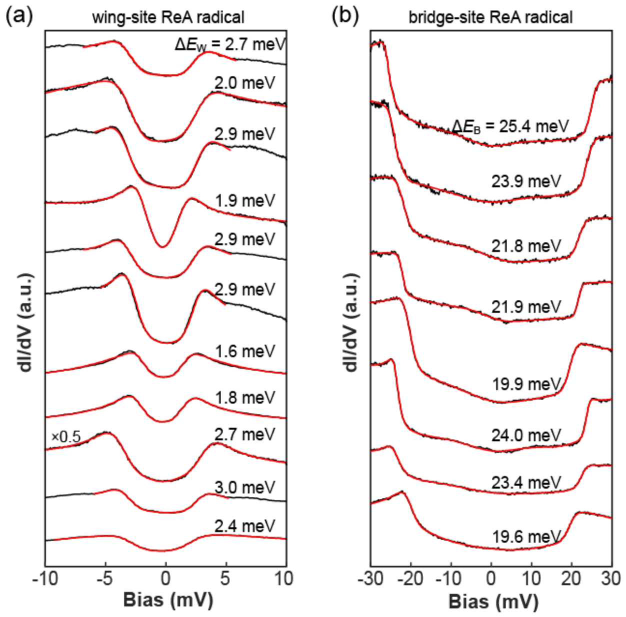


**Fig. S3 Representative *dI/dV* spectra measured on different ReA radicals in the Fe-coordinated tetramers.** (a) Wing-site, (b) Bridge-site. The black lines are experimental data, and the red lines are theoretical fits. The fitted spin excitation energy ($\Delta E_W$ and $\Delta E_B$) is labelled aside each spectrum.

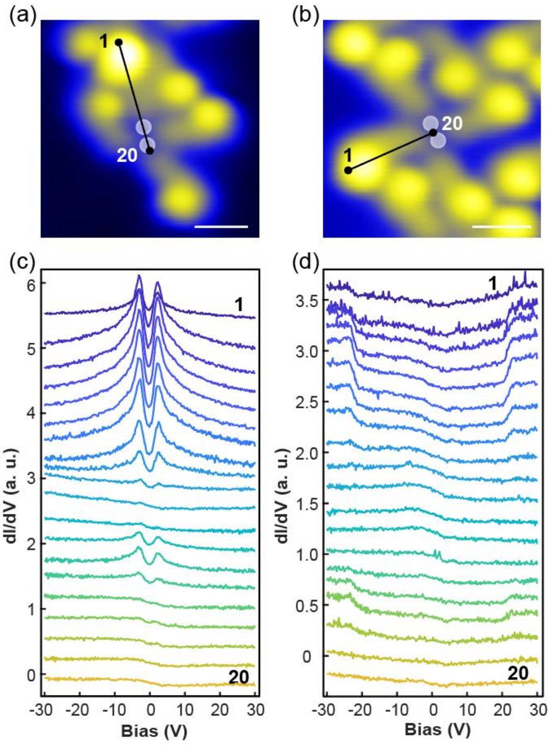


**Fig. S4 *dI/dV* spectra measured at different positions on the ReA radical in the coordinated tetramer.** (a, b) STM images of a coordinated tetramer in which a wing-site (a) and a bridge-site (b) was transformed into a radical, respectively. The black lines along the molecular

skeleton indicate the positions where the *dI/dV* were measured. (c, d) *dI/dV* spectra measured at 20 points equidistantly along the black lines in (a) and (b), respectively. Scanning parameters: constant-current mode, $V_b$ = 30 mV, $I_{set}$ = 53 pA. *dI/dV* parameters: $V_b$ = 30 mV, $I_{set}$ = 200 pA, $V_{mod}$ = 0.6 mV.

## References


[1] G. Kresse and J. Hafner, *Phys. Rev. B* 1993, **47**, 558-561.
[2] G. Kresse and J. Furthmüller, *Phys. Rev. B* 1996, **54**, 11169-11186.
[3] P. E. Blöchl, *Phys. Rev. B* 1994, **50**, 17953-17979.
[4] J. P. Perdew , K. Burke and M. Ernzerhof, *Phys. Rev. Lett.* 1996, **77**, 3865-3868.
[5] S. L. Dudarev, G. A. Botton, S. Y. Savrasov, C. J. Humphreys, A. P. Sutton, *Phys. Rev. B* 1998, **57**, 1505.
[6] S. Grimme, J. Antony, S. Ehrlich and H. Krieg, *J. Chem. Phys.* 2010, **132**, 154104.
[7] E. R. Johnson and A. D. Becke, *J. Chem. Phys.* 2006, **124**, 174104.
[8] M. Ternes, *New J. Phys.* 2015, **17**, 063016.
